# Supplementary material for: Unsupervised Layer-wise Score Aggregation for Textual OOD Detection
Source: arXiv:2302.09852 source file (2024-02-21)
Supplement: Supplementary file 1 [file appendix_perf_per_layer_figcode.tex]

\begin{figure*}\centering\begin{subfigure}[b]{0.45\textwidth}
\includegraphics[width=\textwidth]{ figures/fig1_bert-base-multilingual-uncased_de_xstance_de_pawsx.pdf}
\caption{de_pawsx}
\end{subfigure}\begin{subfigure}[b]{0.45\textwidth}
\includegraphics[width=\textwidth]{ figures/fig1_bert-base-multilingual-uncased_de_xstance_de_swiss_judgement.pdf}
\caption{de_swiss_judgement}
\end{subfigure}
 
\begin{subfigure}[b]{0.45\textwidth}
\includegraphics[width=\textwidth]{ figures/fig1_bert-base-multilingual-uncased_de_xstance_de_tweet_sentiment.pdf}
\caption{de_tweet_sentiment}
\end{subfigure}\caption{OOD detection performance in terms of AUROC for each feature-based OOD score computed at each layer for all Out-DS for bert-base-multilingual-uncased and de_xstance}
\label{fig:perfs_per_layer_bert-base-multilingual-uncasedde_xstance}
\end{figure*}
\begin{figure*}\centering\begin{subfigure}[b]{0.45\textwidth}
\includegraphics[width=\textwidth]{ figures/fig1_bert-base-multilingual-uncased_de_swiss_judgement_de_pawsx.pdf}
\caption{de_pawsx}
\end{subfigure}\begin{subfigure}[b]{0.45\textwidth}
\includegraphics[width=\textwidth]{ figures/fig1_bert-base-multilingual-uncased_de_swiss_judgement_de_tweet_sentiment.pdf}
\caption{de_tweet_sentiment}
\end{subfigure}
 
\begin{subfigure}[b]{0.45\textwidth}
\includegraphics[width=\textwidth]{ figures/fig1_bert-base-multilingual-uncased_de_swiss_judgement_de_xstance.pdf}
\caption{de_xstance}
\end{subfigure}\caption{OOD detection performance in terms of AUROC for each feature-based OOD score computed at each layer for all Out-DS for bert-base-multilingual-uncased and de_swiss_judgement}
\label{fig:perfs_per_layer_bert-base-multilingual-uncasedde_swiss_judgement}
\end{figure*}
\begin{figure*}\centering\begin{subfigure}[b]{0.45\textwidth}
\includegraphics[width=\textwidth]{ figures/fig1_bert-base-multilingual-uncased_de_tweet_sentiment_de_pawsx.pdf}
\caption{de_pawsx}
\end{subfigure}\begin{subfigure}[b]{0.45\textwidth}
\includegraphics[width=\textwidth]{ figures/fig1_bert-base-multilingual-uncased_de_tweet_sentiment_de_swiss_judgement.pdf}
\caption{de_swiss_judgement}
\end{subfigure}
 
\begin{subfigure}[b]{0.45\textwidth}
\includegraphics[width=\textwidth]{ figures/fig1_bert-base-multilingual-uncased_de_tweet_sentiment_de_xstance.pdf}
\caption{de_xstance}
\end{subfigure}\caption{OOD detection performance in terms of AUROC for each feature-based OOD score computed at each layer for all Out-DS for bert-base-multilingual-uncased and de_tweet_sentiment}
\label{fig:perfs_per_layer_bert-base-multilingual-uncasedde_tweet_sentiment}
\end{figure*}
\begin{figure*}\centering\begin{subfigure}[b]{0.45\textwidth}
\includegraphics[width=\textwidth]{ figures/fig1_bert-base-multilingual-uncased_de_pawsx_de_swiss_judgement.pdf}
\caption{de_swiss_judgement}
\end{subfigure}\begin{subfigure}[b]{0.45\textwidth}
\includegraphics[width=\textwidth]{ figures/fig1_bert-base-multilingual-uncased_de_pawsx_de_tweet_sentiment.pdf}
\caption{de_tweet_sentiment}
\end{subfigure}
 
\begin{subfigure}[b]{0.45\textwidth}
\includegraphics[width=\textwidth]{ figures/fig1_bert-base-multilingual-uncased_de_pawsx_de_xstance.pdf}
\caption{de_xstance}
\end{subfigure}\caption{OOD detection performance in terms of AUROC for each feature-based OOD score computed at each layer for all Out-DS for bert-base-multilingual-uncased and de_pawsx}
\label{fig:perfs_per_layer_bert-base-multilingual-uncasedde_pawsx}
\end{figure*}
\begin{figure*}\centering\begin{subfigure}[b]{0.45\textwidth}
\includegraphics[width=\textwidth]{ figures/fig1_bert-base-multilingual-uncased_es_tweet_sentiment_es_cine.pdf}
\caption{es_cine}
\end{subfigure}\begin{subfigure}[b]{0.45\textwidth}
\includegraphics[width=\textwidth]{ figures/fig1_bert-base-multilingual-uncased_es_tweet_sentiment_es_pawsx.pdf}
\caption{es_pawsx}
\end{subfigure}
 
\begin{subfigure}[b]{0.45\textwidth}
\includegraphics[width=\textwidth]{ figures/fig1_bert-base-multilingual-uncased_es_tweet_sentiment_es_tweet_inde.pdf}
\caption{es_tweet_inde}
\end{subfigure}\caption{OOD detection performance in terms of AUROC for each feature-based OOD score computed at each layer for all Out-DS for bert-base-multilingual-uncased and es_tweet_sentiment}
\label{fig:perfs_per_layer_bert-base-multilingual-uncasedes_tweet_sentiment}
\end{figure*}
\begin{figure*}\centering\begin{subfigure}[b]{0.45\textwidth}
\includegraphics[width=\textwidth]{ figures/fig1_bert-base-multilingual-uncased_es_pawsx_es_cine.pdf}
\caption{es_cine}
\end{subfigure}\begin{subfigure}[b]{0.45\textwidth}
\includegraphics[width=\textwidth]{ figures/fig1_bert-base-multilingual-uncased_es_pawsx_es_tweet_inde.pdf}
\caption{es_tweet_inde}
\end{subfigure}
 
\begin{subfigure}[b]{0.45\textwidth}
\includegraphics[width=\textwidth]{ figures/fig1_bert-base-multilingual-uncased_es_pawsx_es_tweet_sentiment.pdf}
\caption{es_tweet_sentiment}
\end{subfigure}\caption{OOD detection performance in terms of AUROC for each feature-based OOD score computed at each layer for all Out-DS for bert-base-multilingual-uncased and es_pawsx}
\label{fig:perfs_per_layer_bert-base-multilingual-uncasedes_pawsx}
\end{figure*}
\begin{figure*}\centering\begin{subfigure}[b]{0.45\textwidth}
\includegraphics[width=\textwidth]{ figures/fig1_bert-base-multilingual-uncased_es_cine_es_pawsx.pdf}
\caption{es_pawsx}
\end{subfigure}\begin{subfigure}[b]{0.45\textwidth}
\includegraphics[width=\textwidth]{ figures/fig1_bert-base-multilingual-uncased_es_cine_es_tweet_inde.pdf}
\caption{es_tweet_inde}
\end{subfigure}
 
\begin{subfigure}[b]{0.45\textwidth}
\includegraphics[width=\textwidth]{ figures/fig1_bert-base-multilingual-uncased_es_cine_es_tweet_sentiment.pdf}
\caption{es_tweet_sentiment}
\end{subfigure}\caption{OOD detection performance in terms of AUROC for each feature-based OOD score computed at each layer for all Out-DS for bert-base-multilingual-uncased and es_cine}
\label{fig:perfs_per_layer_bert-base-multilingual-uncasedes_cine}
\end{figure*}
\begin{figure*}\centering\begin{subfigure}[b]{0.45\textwidth}
\includegraphics[width=\textwidth]{ figures/fig1_bert-base-multilingual-uncased_es_tweet_inde_es_cine.pdf}
\caption{es_cine}
\end{subfigure}\begin{subfigure}[b]{0.45\textwidth}
\includegraphics[width=\textwidth]{ figures/fig1_bert-base-multilingual-uncased_es_tweet_inde_es_pawsx.pdf}
\caption{es_pawsx}
\end{subfigure}
 
\begin{subfigure}[b]{0.45\textwidth}
\includegraphics[width=\textwidth]{ figures/fig1_bert-base-multilingual-uncased_es_tweet_inde_es_tweet_sentiment.pdf}
\caption{es_tweet_sentiment}
\end{subfigure}\caption{OOD detection performance in terms of AUROC for each feature-based OOD score computed at each layer for all Out-DS for bert-base-multilingual-uncased and es_tweet_inde}
\label{fig:perfs_per_layer_bert-base-multilingual-uncasedes_tweet_inde}
\end{figure*}
